# Supplementary material for: CV4Code: Sourcecode Understanding via Visual Code Representations
Source: arXiv:2205.08585 source file (2022-05-11)
Supplement: Supplementary file 1 [file supplementary.tex]

\section{Supplementary material}

We provide additional material to supplement our main submission. In particular, the following aspects are covered:

\begin{itemize}
    \item DeepLPF Parameter Prediction Block Architecture (Section~\ref{sec:dpf_regression_block})
    \item DeepLPF Multiple Filter Fusion Architecture (Section~\ref{sec:dpf_fusion_block})
    \item Additional Qualitative Visual Results (Section~\ref{sec:dpf_visual_examples}) %visual examples 
\end{itemize}

\begin{figure*}[ht]
\includegraphics[scale=0.5]{images/sec3/regressionNN-crop.pdf}
\caption{\textbf{Filter Parameter regression architecture of DeepLPF}. Given features from a backbone network, the parameter regression network infers the parameters of the parametric filters (polynomial, elliptical, or graduated).}
\label{fig:regressionNN}
\end{figure*}

\begin{figure*}[t]
\begin{center}
\includegraphics[scale = 0.3, width=\linewidth]{DPF/images/sec3/PixelBlock2-crop.pdf}
\end{center}
\caption{\textbf{RGB-to-RGB Pixel-level block of DeepLPF}. The block is broadly modelled as a U-Net. The RGB image data is input on the left and the RGB image is output on the right. }
\label{fig:pixel_level2}
\end{figure*}

\subsection{DeepLPF Parameter Prediction Architecture }\label{sec:dpf_regression_block}

Figure~\ref{fig:regressionNN} presents the architecture of the DeepLPF parameter prediction network. The network accepts from the backbone feature extraction neural network (\eg~a U-Net~\cite{Ronneberger15}) a feature map  of dimension $H{\times}W{\times}C$, where $H$ is the height, $W$ is the width and $C$ is the channel count. The extracted features are passed through an alternating series of convolution and maxpooling blocks, followed by a global average pooling and fully connected layer. Leaky ReLUs serve as the activation functions and dropout is employed before the fully connected layer (applied 50\% at both training and test time).

\subsection{DeepLPF Multiple Filter Fusion Architecture}\label{sec:dpf_fusion_block}

Figure~\ref{fig:radialCombine} presents the filter fusion architecture, which receives the scaling maps of multiple filters of the same type (here we show elliptical filters but the same architecture is used for graduated filters) and combines the filters through multiplication into a single scaling map to be applied to the input image to yield the enhanced image. 

\begin{figure}[tbh!]
\
\includegraphics[width=1.0\linewidth]{images/sec3/elliptical_fusion.PNG} 	
%	\vskip -0.2cm
\caption{\textbf{Fusion architecture} for several instances of the elliptical filter.}
\label{fig:radialCombine}
%\vspace{-0.3cm}
\end{figure}

\subsection{Additional Visual Examples}\label{sec:dpf_visual_examples}

Further filter visualizations, output image examples from DeepLPF and the baseline models on the SID and Adobe datasets are presented in Figures~\ref{fig:visual_comparison1}-\ref{fig:graduated}:

\begin{itemize}
    \item Figure~\ref{fig:visual_comparison1}: Comparison between DeepLPF and DeepUPE~\cite{wang2019underexposed} on sample images from the MIT-Adobe5k-UPE dataset.
      \item Figure~\ref{fig:visual_comparison3b}: Additional qualitative comparison between DeepLPF and DPE~\cite{chen2018deep} on sample images of the MIT-Adobe5k-DPE dataset.
        \item Figure~\ref{fig:visual_comparison4}: Qualitative comparison between DeepLPF and SID~\cite{chen2018learning} architecture on sample images of the Fuji partition of the SID dataset.     
    \item Figure~\ref{fig:visual_comparison5}: Additional visual results from the MIT-Adobe5k-DPE dataset comparing DeepLPF to DPE\cite{chen2018deep}, CLHE\cite{Wang17}, DPED (iphone7)\cite{ignatov2017dslr}, NPEA\cite{Gao17}, FLLF\cite{Aubry14}
        \item Figure~\ref{fig:visual_comparison6}: Additional visual results from the MIT-Adobe5k-DPE dataset comparing DeepLPF to DPE\cite{chen2018deep}, CLHE\cite{Wang17}, DPED (iphone7)\cite{ignatov2017dslr}, NPEA\cite{Gao17}, FLLF\cite{Aubry14}
            \item Figure~\ref{fig:visual_comparison7}: Additional qualitative comparison on sample images from the MIT-Adobe5k-DPE dataset.
    \item Figure~\ref{fig:ablation5}: Ablation study showing the effect of different combinations of parametric filter compared to the groundtruth and the baseline U-Net~\cite{Ronneberger15} on the Adobe5k-DPE dataset.
    \item Figure~\ref{fig:limitations}:  Examples of DeepLPF failure cases. 
    \item Figure~\ref{fig:elliptical}:  Additional examples of elliptical filters acting on different channels of the input images.
    \item Figure~\ref{fig:graduated}: Additional examples of mixtures of graduated or elliptical filters acting on different channels of the input images.
\end{itemize}

\begin{figure*}[t!]
\begin{center}
\begin{tabular}{c@{}c@{}c@{}c@{}}
\scalebox{0.85}{Input} &
\scalebox{0.85}{DeepUPE~\cite{wang2019underexposed}} & 
\scalebox{0.85}{\textbf{DeepLPF} } &
\scalebox{0.85}{Ground Truth} \\
\includegraphics[scale=0.30205]{DPF/images/sec4/Adobe_UPE/a4922_input.jpg}&
\includegraphics[scale=0.121]{DPF/images/sec4/Adobe_UPE/a4922_png_npy.png}&
\includegraphics[scale=0.068]{DPF/images/sec4/Adobe_UPE/a4922.jpg}&
\includegraphics[scale=0.126]{DPF/images/sec4/Adobe_UPE/truth_a4922.jpg}\\
\end{tabular}

\begin{tabular}{c@{}c@{}c@{}c@{}}
\includegraphics[scale=0.452]{DPF/images/sec4/Adobe_UPE/a4972_input.jpg}&
\includegraphics[scale=0.0805]{DPF/images/sec4/Adobe_UPE/a4972_png_npy.png}&
\includegraphics[scale=0.084]{DPF/images/sec4/Adobe_UPE/a4972.jpg}&
\includegraphics[scale=0.084]{DPF/images/sec4/Adobe_UPE/truth_a4972.jpg} \\
\end{tabular}

\begin{tabular}{c@{}c@{}c@{}c@{}}
\includegraphics[scale=0.682]{DPF/images/sec4/Adobe_UPE/a4980_input.jpg}&
\includegraphics[scale=0.121]{DPF/images/sec4/Adobe_UPE/a4980_png_npy.png}&
\includegraphics[scale=0.126]{DPF/images/sec4/Adobe_UPE/a4980.jpg}&
\includegraphics[scale=0.126]{DPF/images/sec4/Adobe_UPE/truth_a4980.jpg}\\
\end{tabular}

\begin{tabular}{c@{}c@{}c@{}c@{}}
\includegraphics[scale=0.452]{DPF/images/sec4/Adobe_UPE/a4985_input.jpg}&
\includegraphics[scale=0.0805]{DPF/images/sec4/Adobe_UPE/a4985_png_npy.png}&
\includegraphics[scale=0.084]{DPF/images/sec4/Adobe_UPE/a4985.jpg}&
\includegraphics[scale=0.084]{DPF/images/sec4/Adobe_UPE/truth_a4985.jpg}\\
\end{tabular}

\end{center}
\caption{Additional qualitative comparison between \textbf{DeepLPF} and \textbf{DeepUPE} on sample images from the \textbf{MIT-Adobe5k-UPE} dataset.}
\label{fig:visual_comparison1}
\end{figure*}

% \begin{figure*}[t]
% \begin{center}

% \begin{tabular}{c@{}c@{}c@{}c@{}}
% \scalebox{0.85}{Input} &
% \scalebox{0.85}{U-Net} & 
% \scalebox{0.85}{DeepLPF } &
% \scalebox{0.85}{Ground Truth} \\
% \includegraphics[scale=0.53]{DPF/images/sec4/Adobe_UPE/a4536_input.jpg}&
% \includegraphics[scale=0.22]{DPF/images/sec4/Adobe_UPE/net_out_TEST_75_6.jpg}&
% \includegraphics[scale=0.22]{DPF/images/sec4/Adobe_UPE/a4536.jpg}&
% \includegraphics[scale=0.22]{DPF/images/sec4/Adobe_UPE/truth_a4536.jpg}\\
% \end{tabular}

% \begin{tabular}{c@{}c@{}c@{}c@{}}
% \includegraphics[scale=0.53]{DPF/images/sec4/Adobe_UPE/a4868_input.jpg}&
% \includegraphics[scale=0.22]{DPF/images/sec4/Adobe_UPE/net_out_TEST_75_4.jpg}&
% \includegraphics[scale=0.22]{DPF/images/sec4/Adobe_UPE/a4868.jpg}&
% \includegraphics[scale=0.22]{DPF/images/sec4/Adobe_UPE/truth_a4868.jpg}\\
% \end{tabular}

% \end{center}
% \caption{Additional qualitative comparison considering both the baseline \textbf{U-Net} and \textbf{DeepLPF} on two samples from the \textbf{MIT-Adobe5k-UPE} dataset. \sean{Remove this as differences not compelling enough?} \steven{agree.}}
% \label{fig:visual_comparison2}
% \end{figure*}

\begin{figure*}[t]
\begin{center}

\begin{tabular}{c@{}c@{}c@{}c@{}}
    \scalebox{0.85}{Input} &
      \scalebox{0.85}{DPE~\cite{chen2018deep}} & 
      \scalebox{0.85}{\textbf{DeepLPF} } &
      \scalebox{0.85}{Ground Truth} \\
     \includegraphics[scale=0.194]{DPF/images/sec4/Adobe_DPE/a1954_input.jpg} &
\includegraphics[scale=0.1835]{DPF/images/sec4/Adobe_DPE/a1954.png} &
\includegraphics[scale=0.191]{DPF/images/sec4/Adobe_DPE/net_out_TEST_250_21.jpg} &
\includegraphics[scale=0.191]{DPF/images/sec4/Adobe_DPE/truth_TEST_299_21.jpg}\\
\end{tabular}

% \begin{tabular}{c@{}c@{}c@{}c@{}}
% \includegraphics[scale=0.192]{DPF/images/sec4/Adobe_DPE/a0905_input.jpg} &
% \includegraphics[scale=0.1835]{DPF/images/sec4/Adobe_DPE/a0905.png} &
% \includegraphics[scale=0.191]{DPF/images/sec4/Adobe_DPE/net_out_TEST_250_2.jpg} &
% \includegraphics[scale=0.191]{DPF/images/sec4/Adobe_DPE/truth_TEST_299_2.jpg}\\
% \end{tabular}

\begin{tabular}{c@{}c@{}c@{}c@{}}
\includegraphics[scale=0.193]{DPF/images/sec4/Adobe_DPE/a2095_input.jpg} &
\includegraphics[scale=0.1835]{DPF/images/sec4/Adobe_DPE/a2095.png} &
\includegraphics[scale=0.191]{DPF/images/sec4/Adobe_DPE/net_out_TEST_250_24.jpg} &
\includegraphics[scale=0.191]{DPF/images/sec4/Adobe_DPE/truth_TEST_299_24.jpg}\\
\end{tabular}

\begin{tabular}{c@{}c@{}c@{}c@{}}
\includegraphics[scale=0.182]{DPF/images/sec4/Adobe_DPE/a0759_input.jpg} &
\includegraphics[scale=0.1835]{DPF/images/sec4/Adobe_DPE/a0759.png} &
\includegraphics[scale=0.191]{DPF/images/sec4/Adobe_DPE/a0759_TEST_2_106.jpg} &
\includegraphics[scale=0.191]{DPF/images/sec4/Adobe_DPE/truth_TEST_1_106.jpg}\\
\end{tabular}

% \begin{tabular}{c@{}c@{}c@{}c@{}}
% \includegraphics[scale=0.293]{DPF/images/sec4/Adobe_DPE/a4504_input.jpg} &
% \includegraphics[scale=0.278]{DPF/images/sec4/Adobe_DPE/a4504.png} &
% \includegraphics[scale=0.290]{DPF/images/sec4/Adobe_DPE/net_out_TEST_250_12.jpg} &
% \includegraphics[scale=0.290]{DPF/images/sec4/Adobe_DPE/truth_TEST_299_12.jpg}\\
% \end{tabular}

\end{center}
\caption{Additional qualitative comparison between \textbf{DeepLPF} and \textbf{DPE}~\cite{chen2018deep} on sample images of the \textbf{MIT-Adobe5k-DPE} dataset.}
\label{fig:visual_comparison3b}
\end{figure*}

\begin{figure*}[t]
\begin{center}

\begin{tabular}{c@{}c@{}c@{}c@{}}
    \scalebox{0.85}{Input} &
      \scalebox{0.85}{U-Net~\cite{Ronneberger15}} & 
      \scalebox{0.85}{\textbf{DeepLPF} } &
      \scalebox{0.85}{Ground Truth} \\
     \includegraphics[scale=0.184]{DPF/images/sec4/Adobe_DPE/a2939_input.jpg} &
\includegraphics[scale=0.191]{DPF/images/sec4/Adobe_DPE/unet_out_TEST_75_1.jpg} &
\includegraphics[scale=0.191]{DPF/images/sec4/Adobe_DPE/net_out_TEST_250_1.jpg} &
\includegraphics[scale=0.191]{DPF/images/sec4/Adobe_DPE/truth_TEST_299_1.jpg}\\
\end{tabular}

\begin{tabular}{c@{}c@{}c@{}c@{}}
\includegraphics[scale=0.184]{DPF/images/sec4/Adobe_DPE/a3245_input.jpg} &
\includegraphics[scale=0.191]{DPF/images/sec4/Adobe_DPE/unet_out_TEST_75_3.jpg} &
\includegraphics[scale=0.191]{DPF/images/sec4/Adobe_DPE/net_out_TEST_250_3.jpg} &
\includegraphics[scale=0.191]{DPF/images/sec4/Adobe_DPE/truth_TEST_299_3.jpg}\\
\end{tabular}

\begin{tabular}{c@{}c@{}c@{}c@{}}
\includegraphics[scale=0.280]{DPF/images/sec4/Adobe_DPE/a4256_input.jpg} &
\includegraphics[scale=0.290]{DPF/images/sec4/Adobe_DPE/unet_out_TEST_75_5.jpg} &
\includegraphics[scale=0.290]{DPF/images/sec4/Adobe_DPE/net_out_TEST_250_5.jpg} &
\includegraphics[scale=0.290]{DPF/images/sec4/Adobe_DPE/truth_TEST_299_5.jpg}\\
\end{tabular}

% \begin{tabular}{c@{}c@{}c@{}c@{}}
% \includegraphics[scale=0.293]{DPF/images/sec4/Adobe_DPE/a0688_input.jpg} &
% \includegraphics[scale=0.278]{DPF/images/sec4/Adobe_DPE/unet_out_TEST_75_8.jpg} &
% \includegraphics[scale=0.290]{DPF/images/sec4/Adobe_DPE/net_out_TEST_250_8.jpg} &
% \includegraphics[scale=0.290]{DPF/images/sec4/Adobe_DPE/truth_TEST_299_8.jpg}\\
% \end{tabular}

\begin{tabular}{c@{}c@{}c@{}c@{}}
\includegraphics[scale=0.184]{DPF/images/sec4/Adobe_DPE/a2369_input.jpg} &
\includegraphics[scale=0.191]{DPF/images/sec4/Adobe_DPE/unet_out_TEST_75_22.jpg} &
\includegraphics[scale=0.191]{DPF/images/sec4/Adobe_DPE/net_out_TEST_250_22.jpg} &
\includegraphics[scale=0.191]{DPF/images/sec4/Adobe_DPE/truth_TEST_299_22.jpg}\\
\end{tabular}

\end{center}
\caption{Additional qualitative comparison between the baseline \textbf{U-Net}~\cite{Ronneberger15} and \textbf{DeepLPF} on sample images from the \textbf{MIT-Adobe5k-DPE} dataset.}
\label{fig:visual_comparison4}
\end{figure*}

\begin{figure*}[t]
\begin{center}

\begin{tabular}{c@{}c@{}c@{}c@{}}
    \scalebox{0.85}{Input} &
      \scalebox{0.85}{DPE~\cite{chen2018deep}} & 
      \scalebox{0.85}{\textbf{DeepLPF} } &
      \scalebox{0.85}{Ground Truth} \\
      \includegraphics[scale=0.300]{DPF/images/sec4/Adobe_DPE/a3203_input.jpg} &
      \includegraphics[scale=0.284]{DPF/images/sec4/Adobe_DPE/a3203.png} &
      \includegraphics[scale=0.296]{DPF/images/sec4/Adobe_DPE/net_out_TEST_250_23.jpg} &
      \includegraphics[scale=0.296]{DPF/images/sec4/Adobe_DPE/truth_TEST_299_23.jpg}\\
\end{tabular}

\begin{tabular}{c@{}c@{}c@{}c@{}}
    \scalebox{0.85}{CLHE~\cite{Wang17}} &
      \scalebox{0.85}{DPED (iphone7)~\cite{ignatov2017dslr}} & 
      \scalebox{0.85}{NPEA~\cite{Gao17}} &
      \scalebox{0.85}{FLLF~\cite{Aubry14}} \\
      \includegraphics[scale=0.290]{DPF/images/sec4/Adobe_DPE/a3203_clhe.png} &
      \includegraphics[scale=0.291]{DPF/images/sec4/Adobe_DPE/a3203_dped.png} &
      \includegraphics[scale=0.290]{DPF/images/sec4/Adobe_DPE/a3203_npea.png} &
      \includegraphics[scale=0.290]{DPF/images/sec4/Adobe_DPE/a3203_fllf.png}\\
\end{tabular}

\begin{tabular}{c@{}c@{}c@{}c@{}}
    \scalebox{0.85}{Input} &
      \scalebox{0.85}{DPE~\cite{chen2018deep}} & 
      \scalebox{0.85}{\textbf{DeepLPF} } &
      \scalebox{0.85}{Ground Truth} \\
      \includegraphics[scale=0.2]{DPF/images/sec4/Adobe_DPE/a3451_input.png} &
      \includegraphics[scale=0.2]{DPF/images/sec4/Adobe_DPE/a3451_dpe.png} &
      \includegraphics[scale=0.208]{DPF/images/sec4/Adobe_DPE/a3451_TEST_2_48.jpg} &
      \includegraphics[scale=0.2]{DPF/images/sec4/Adobe_DPE/a3451_gt.png}\\
\end{tabular}

\begin{tabular}{c@{}c@{}c@{}c@{}}
    \scalebox{0.85}{CLHE~\cite{Wang17}} &
      \scalebox{0.85}{DPED (iphone7)~\cite{ignatov2017dslr}} & 
      \scalebox{0.85}{NPEA~\cite{Gao17}} &
      \scalebox{0.85}{FLLF~\cite{Aubry14}} \\
      \includegraphics[scale=0.2]{DPF/images/sec4/Adobe_DPE/a3451_clhe.png} &
      \includegraphics[scale=0.2]{DPF/images/sec4/Adobe_DPE/a3451_dped.png} &
      \includegraphics[scale=0.2]{DPF/images/sec4/Adobe_DPE/a3451_npea.png} &
      \includegraphics[scale=0.2]{DPF/images/sec4/Adobe_DPE/a3451_fllf.png}\\
\end{tabular}

\end{center}
\caption{Additional visual results from the MIT-Adobe5k-DPE dataset comparing \textbf{DeepLPF} to \textbf{DPE}~\cite{chen2018deep}, \textbf{CLHE}~\cite{Wang17}, \textbf{DPED (iphone7)}~\cite{ignatov2017dslr}, \textbf{NPEA}~\cite{Gao17}, \textbf{FLLF}~\cite{Aubry14}}
\label{fig:visual_comparison5}
\end{figure*}

\begin{figure*}[t]
\begin{center}

\begin{tabular}{c@{}c@{}c@{}c@{}}
    \scalebox{0.85}{Input} &
      \scalebox{0.85}{DPE~\cite{chen2018deep}} & 
      \scalebox{0.85}{\textbf{DeepLPF} } &
      \scalebox{0.85}{Ground Truth} \\
      \includegraphics[scale=0.2]{DPF/images/sec4/Adobe_DPE/a0535_input.png} &
      \includegraphics[scale=0.2]{DPF/images/sec4/Adobe_DPE/a0535_dpe.png} &
      \includegraphics[scale=0.208]{DPF/images/sec4/Adobe_DPE/a0535_TEST_2_269.jpg} &
      \includegraphics[scale=0.2]{DPF/images/sec4/Adobe_DPE/a0535_gt.png}\\
\end{tabular}

\begin{tabular}{c@{}c@{}c@{}c@{}}
    \scalebox{0.85}{CLHE~\cite{Wang17}} &
      \scalebox{0.85}{DPED (iphone7)~\cite{ignatov2017dslr}} & 
      \scalebox{0.85}{NPEA~\cite{Gao17}} &
      \scalebox{0.85}{FLLF~\cite{Aubry14}} \\
      \includegraphics[scale=0.2]{DPF/images/sec4/Adobe_DPE/a0535_clhe.png} &
      \includegraphics[scale=0.2]{DPF/images/sec4/Adobe_DPE/a0535_dped.png} &
      \includegraphics[scale=0.2]{DPF/images/sec4/Adobe_DPE/a0535_npea.png} &
      \includegraphics[scale=0.2]{DPF/images/sec4/Adobe_DPE/a0535_fllf.png}\\
\end{tabular}

\begin{tabular}{c@{}c@{}c@{}c@{}}
    \scalebox{0.85}{Input} &
      \scalebox{0.85}{DPE~\cite{chen2018deep}} & 
      \scalebox{0.85}{\textbf{DeepLPF} } &
      \scalebox{0.85}{Ground Truth} \\
      \includegraphics[scale=0.2]{DPF/images/sec4/Adobe_DPE/a1305_input.png} &
      \includegraphics[scale=0.2]{DPF/images/sec4/Adobe_DPE/a1305_dpe.png} &
      \includegraphics[scale=0.208]{DPF/images/sec4/Adobe_DPE/a1305_TEST_2_52.jpg} &
      \includegraphics[scale=0.2]{DPF/images/sec4/Adobe_DPE/a1305_gt.png}\\
\end{tabular}

\begin{tabular}{c@{}c@{}c@{}c@{}}
    \scalebox{0.85}{CLHE~\cite{Wang17}} &
      \scalebox{0.85}{DPED (iphone7)~\cite{ignatov2017dslr}} & 
      \scalebox{0.85}{NPEA~\cite{Gao17}} &
      \scalebox{0.85}{FLLF~\cite{Aubry14}} \\
      \includegraphics[scale=0.2]{DPF/images/sec4/Adobe_DPE/a1305_clhe.png} &
      \includegraphics[scale=0.2]{DPF/images/sec4/Adobe_DPE/a1305_dped.png} &
      \includegraphics[scale=0.2]{DPF/images/sec4/Adobe_DPE/a1305_npea.png} &
      \includegraphics[scale=0.2]{DPF/images/sec4/Adobe_DPE/a1305_fllf.png}\\
\end{tabular}

\begin{tabular}{c@{}c@{}c@{}c@{}}
    \scalebox{0.85}{Input} &
      \scalebox{0.85}{DPE~\cite{chen2018deep}} & 
      \scalebox{0.85}{\textbf{DeepLPF} } &
      \scalebox{0.85}{Ground Truth} \\
      \includegraphics[scale=0.2]{DPF/images/sec4/Adobe_DPE/a2995_input.png} &
      \includegraphics[scale=0.2]{DPF/images/sec4/Adobe_DPE/a2995_dpe.png} &
      \includegraphics[scale=0.2085]{DPF/images/sec4/Adobe_DPE/a2995_TEST_2_341.jpg} &
      \includegraphics[scale=0.5]{DPF/images/sec4/Adobe_DPE/a2995_gt.png}\\
\end{tabular}

\begin{tabular}{c@{}c@{}c@{}c@{}}
    \scalebox{0.85}{CLHE~\cite{Wang17}} &
      \scalebox{0.85}{DPED (iphone7)~\cite{ignatov2017dslr}} & 
      \scalebox{0.85}{NPEA~\cite{Gao17}} &
      \scalebox{0.85}{FLLF~\cite{Aubry14}} \\
      \includegraphics[scale=0.2]{DPF/images/sec4/Adobe_DPE/a2995_clhe.png} &
      \includegraphics[scale=0.15]{DPF/images/sec4/Adobe_DPE/a2995_dped.png} &
      \includegraphics[scale=0.2]{DPF/images/sec4/Adobe_DPE/a2995_npea.png} &
      \includegraphics[scale=0.2]{DPF/images/sec4/Adobe_DPE/a2995_fllf.png}\\
\end{tabular}

\end{center}
\caption{Additional visual results from the MIT-Adobe5k-DPE dataset comparing \textbf{DeepLPF} to \textbf{DPE}~\cite{chen2018deep}, \textbf{CLHE}~\cite{Wang17}, \textbf{DPED (iphone7)}~\cite{ignatov2017dslr}, \textbf{NPEA}~\cite{Gao17}, \textbf{FLLF}~\cite{Aubry14}}
\label{fig:visual_comparison6}
\end{figure*}

\begin{figure*}[t]
\begin{center}

\begin{tabular}{c@{}c@{}c@{}}
\scalebox{0.85}{SID~\cite{chen2018learning}} & 
\scalebox{0.85}{\textbf{DeepLPF} } &
\scalebox{0.85}{Ground Truth} \\
\includegraphics[width=0.33\linewidth]{DPF/images/sec4/SID/10019_00_100_out.png}&
\includegraphics[width=0.33\linewidth]{DPF/images/sec4/SID/10019_00_0.jpg}&
\includegraphics[width=0.33\linewidth]{DPF/images/sec4/SID/10019_00_100_gt.png}\\
\end{tabular}

\begin{tabular}{c@{}c@{}c@{}}
\includegraphics[width=0.33\linewidth]{DPF/images/sec4/SID/10027_00_100_out.png}&
\includegraphics[width=0.33\linewidth]{DPF/images/sec4/SID/10027_00_0.jpg}&
\includegraphics[width=0.33\linewidth]{DPF/images/sec4/SID/10027_00_100_gt.png}\\
\end{tabular}

\begin{tabular}{c@{}c@{}c@{}}
\includegraphics[width=0.33\linewidth]{DPF/images/sec4/SID/10051_00_100_out.png}&
\includegraphics[width=0.33\linewidth]{DPF/images/sec4/SID/10051_00_0.jpg}&
\includegraphics[width=0.33\linewidth]{DPF/images/sec4/SID/10051_00_100_gt.png}\\
\end{tabular}

\begin{tabular}{c@{}c@{}c@{}}
\includegraphics[width=0.33\linewidth]{DPF/images/sec4/SID/10145_00_100_out.png}&
\includegraphics[width=0.33\linewidth]{DPF/images/sec4/SID/10145_00_0.jpg}&
\includegraphics[width=0.33\linewidth]{DPF/images/sec4/SID/10145_00_100_gt.png}\\
\end{tabular}

\begin{tabular}{c@{}c@{}c@{}}
\includegraphics[width=0.33\linewidth]{DPF/images/sec4/SID/10134_00_100_out.png}&
\includegraphics[width=0.33\linewidth]{DPF/images/sec4/SID/10134_00_0_1_PSNR_33_222_SSIM_0_917.jpg}&
\includegraphics[width=0.33\linewidth]{DPF/images/sec4/SID/10134_00_100_gt.png}\\
\end{tabular}

\end{center}
\caption{Qualitative comparison between \textbf{DeepLPF} and \textbf{SID}~\cite{chen2018learning} on sample images of the Fuji partition of the \textbf{SID} dataset.}
\label{fig:visual_comparison7}
\end{figure*}

% \begin{figure*}[t]
% \begin{center}

% \begin{tabular}{c@{}c@{}c@{}}
% \scalebox{0.85}{SID} & 
% \scalebox{0.85}{\textbf{DeepLPF} } &
% \scalebox{0.85}{Ground Truth} \\
% \includegraphics[scale=0.3]{DPF/images/sec4/SID/10133_00_100_out.png}&
% \includegraphics[scale=0.313]{DPF/images/sec4/SID/10133_00_0.jpg}&
% \includegraphics[scale=0.3]{DPF/images/sec4/SID/10133_00_100_gt.png}&\\
% \end{tabular}

% \begin{tabular}{c@{}c@{}c@{}}
% \includegraphics[scale=0.3]{DPF/images/sec4/SID/10145_00_100_out.png}&
% \includegraphics[scale=0.3125]{DPF/images/sec4/SID/10145_00_0.jpg}&
% \includegraphics[scale=0.3]{DPF/images/sec4/SID/10145_00_100_gt.png}&\\
% \end{tabular}

% \end{center}
% \caption{Qualitative comparison between \textbf{DeepLPF} and \textbf{SID architecture} ?? on sample images of the Fuji partition of the textbf{SID} dataset.}
% \label{fig:visual_comparison3}
% \end{figure*}

\begin{figure*}[t!]
\begin{center}
\begin{tabular}{lll}
\begin{subfigure}{0.3\textwidth}
      \centering
      \includegraphics[scale=0.29]{DPF/images/sec4/ablation_input_28.jpg}
      \caption{Input}
\end{subfigure}
\begin{subfigure}{0.3\textwidth}
      \centering
      \includegraphics[scale=0.4]{DPF/images/sec4/ablation_unet_28.jpg}
      \caption{U-Net}
\end{subfigure}
\begin{subfigure}{0.3\textwidth}
      \centering
      \includegraphics[scale=0.4]{{DPF/images/sec4/ablation_rad_28.jpg}}
      \caption{U-Net+Elliptical}
\end{subfigure}
\end{tabular}
\begin{tabular}{lll}
\begin{subfigure}{0.3\textwidth}
      \centering
      \includegraphics[scale=0.4]{DPF/images/sec4/ablation_grad_28.jpg}
      \caption{U-Net+Graduated}
\end{subfigure}
\begin{subfigure}{0.3\textwidth}
      \centering
      \includegraphics[scale=0.4]{DPF/images/sec4/ablation_rad_grad_28.jpg}
      \caption{U-Net+Elliptical+Graduated}
\end{subfigure}
\begin{subfigure}{0.3\textwidth}
      \centering
      \includegraphics[scale=0.4]{{DPF/images/sec4/ablation_cubic_28.jpg}}
      \caption{U-Net+Cubic}
\end{subfigure}
\end{tabular}
\begin{tabular}{lll}
\begin{subfigure}{0.3\textwidth}
      \centering
      \includegraphics[scale=0.4]{{DPF/images/sec4/ablation_full_28.jpg}}
      \caption{U-Net+Cubic+Elliptical+Grad}
\end{subfigure}
\begin{subfigure}{0.3\textwidth}
      \centering
      \includegraphics[scale=0.4]{DPF/images/sec4/ablation_gt_28.jpg}
      \caption{Ground Truth}
\end{subfigure}
\end{tabular}
\end{center}
\caption{Ablation study showing the effect of different combinations of parametric filter compared to the groundtruth and the baseline U-Net~\cite{Ronneberger15} on the \textbf{MIT-Adobe5k-DPE} dataset.}
\label{fig:ablation5}
\end{figure*}

\begin{figure*}[t!]
\begin{center}

\begin{tabular}{c@{}c@{}c@{}c@{}}
    \scalebox{0.85}{Input} &
      \scalebox{0.85}{\textbf{DeepLPF} } &
      \scalebox{0.85}{Ground Truth} \\
\includegraphics[scale=0.355]{DPF/images/sec4/Adobe_DPE/a3203_input.jpg} &
\includegraphics[scale=0.35]{DPF/images/sec4/Adobe_DPE/net_out_TEST_250_23.jpg} &
\includegraphics[scale=0.35]{DPF/images/sec4/Adobe_DPE/truth_TEST_299_23.jpg}\\
\end{tabular}

\begin{tabular}{c@{}c@{}c@{}c@{}}
\includegraphics[scale=0.337]{DPF/images/sec4/Adobe_DPE/a0427_input.jpg} &
\includegraphics[scale=0.35]{DPF/images/sec4/Adobe_DPE/net_out_TEST_250_26.jpg} &
\includegraphics[scale=0.35]{DPF/images/sec4/Adobe_DPE/truth_TEST_299_26.jpg}\\
\end{tabular}

\end{center}
\caption{Example images showing some \textbf{DeepLPF failure cases} with respect to the groundtruth. \textbf{Top:} It can be observed from the training set distribution that our model has likely learned to brighten human faces. The transformation between the input and groundtruth in this example is uncommon in the MIT-Adobe5k dataset as artists generally lighten human faces. We note, however, that DeepLPF has removed the reddish colour cast from the input. \textbf{Bottom:} Here Artist C increases the saturation of the green hue, however DeepLPF fails to match the same level of saturation. This could be addressed by learning the filters in the Hue-Saturation-Value (HSV) colour space, in which the saturation for a particular hue could be precisely adjusted.}
\label{fig:limitations}
\end{figure*}

\begin{figure*}[t!]
\begin{center}
\includegraphics[scale=0.51]{DPF/images/sec1/fig1_3.PNG} \\
\includegraphics[scale=1.15]{DPF/images/sec4/filters/elliptical_1.PNG} \\
\includegraphics[scale=1.16]{DPF/images/sec4/filters/elliptical_2.PNG} \\
\includegraphics[scale=1]{DPF/images/sec4/filters/elliptical_3.PNG}
\end{center}
\caption{Additional examples of elliptical filters acting on different channels of the input images.  \textbf{Left:} Examples of estimated filters. \textbf{Right:} The produced output images.}
\label{fig:elliptical}
\end{figure*}

\begin{figure*}[t!]
\begin{center}
\includegraphics[scale=1.15]{DPF/images/sec4/filters/graduated_1.PNG} \\
\includegraphics[scale=1.15]{DPF/images/sec4/filters/graduated_2.PNG} \\
\includegraphics[scale=1.15]{DPF/images/sec4/filters/elliptical_5.PNG} \\
\end{center}
\caption{Additional examples of mixtures of graduated or elliptical filters acting on different channels of the input images.  \textbf{Left:} Examples of estimated filters. \textbf{Right:} The produced output images.}
\label{fig:graduated}
\end{figure*}
